# Supplementary material for: FreeCHR: An Algebraic Framework for CHR-Embeddings
Source: arXiv:2306.00642 source file (2025-03-19)
Supplement: Supplementary file 1 [file gcd.tex]

\section{Complete proof tree of \autoref{ex:freechr:gcd:exec}}\label{appendix:examples}
Shown below is the complete proof of the derivation $\left\{12, 9\right\} \xmapsto{zero \chrcomp subtract} \left\{3\right\}$ described in \autoref{ex:freechr:gcd:exec}.
\begin{center}
    \begin{prooftree}[small]
        \hypo{0 = 0 \wedge \btrue \equiv \btrue}
        \infer1[apply]{%
            \left\{3, 0\right\} \uplus \emptyset
            \xmapsto{zero}
            \left\{3\right\} \uplus \emptyset \uplus \emptyset}

        \infer0[pass/final]{\left\{3\right\} \xmapsto{zero \chrcomp subtract} \left\{3\right\}}

        \infer2[step$_2$]{\left\{3, 0\right\} \xmapsto{zero \chrcomp subtract} \left\{3\right\}}
    \end{prooftree}

    \bigskip    

    \begin{prooftree}[small]
        \hypo{0 < 3 \wedge 0 < 3 \wedge 3 \leq 3 \equiv \btrue}
        \infer1[apply]{%
            \left\{3, 6\right\} \uplus \emptyset \xmapsto{subtract} \left\{3\right\} \uplus \left\{0\right\} \uplus \emptyset}

        \hypo{\left\{3, 0\right\} \xmapsto{zero \chrcomp subtract} \left\{3\right\}}

        \infer2[step$_2$]{\left\{3, 3\right\} \xmapsto{zero \chrcomp subtract} \left\{3\right\}}
    \end{prooftree}

    \bigskip

    \begin{prooftree}[small]
        \hypo{0 < 3 \wedge 0 < 6 \wedge 3 \leq 6 \equiv \btrue}
        \infer1[apply]{%
            \left\{3, 6\right\} \uplus \emptyset \xmapsto{subtract} \left\{3\right\} \uplus \left\{3\right\} \uplus \emptyset}

        \hypo{\left\{3, 3\right\} \xmapsto{zero \chrcomp subtract} \left\{3\right\}}
        
        \infer2[step$_2$]{\left\{3, 6\right\} \xmapsto{zero \chrcomp subtract} \left\{3\right\}}
    \end{prooftree}

    \bigskip

    \begin{prooftree}[small]
    \hypo{0 < 3 \wedge 0 < 9 \wedge 3 \leq 9 \equiv \btrue}
        \infer1[apply]{%
            \left\{3, 9\right\} \uplus \emptyset \xmapsto{subtract} \left\{3\right\} \uplus \left\{6\right\} \uplus \emptyset}
        
        \hypo{\left\{3, 6\right\} \xmapsto{zero \chrcomp subtract} \left\{3\right\}}

        \infer2[step$_2$]{\left\{3, 9\right\} \xmapsto{zero \chrcomp subtract} \left\{3\right\}}
    \end{prooftree}

    \bigskip

    \begin{prooftree}[small]
        \hypo{0 < 9 \wedge 0 < 12 \wedge 9 \leq 12 \equiv \btrue}
        \infer1[apply]{%
            \left\{12, 9\right\} \uplus \emptyset
            \xmapsto{subtract}
            \left\{9\right\} \uplus \left\{3\right\} \uplus \emptyset}

        \hypo{\left\{3, 9\right\} \xmapsto{zero \chrcomp subtract} \left\{3\right\}}

        \infer2[step$_2$]{%
            \left\{12, 9\right\}
            \xmapsto{zero \chrcomp subtract}
            \left\{3\right\}}
    \end{prooftree}
\end{center}
